# Supplementary material for: Geometric and Nonequilibrium Criticality in Run-and-Tumble Particles with Competing Motility and Attraction
Source: arXiv:2506.05264 source file (2025-10-21)
Supplement: Supplementary file 1 [file supplement.pdf]

# Supplementary Material for “Geometric and Nonequilibrium Criticality in Run-and-Tumble Particles with Competing Motility and Attraction”

Abir Bhowmick,<sup>\*</sup> Sayantan Mitra,<sup>†</sup> and P. K. Mohanty<sup>‡</sup>

*Department of Physical Sciences, Indian Institute of Science Education and Research Kolkata, Mohanpur, 741246 India.*

In this supplemental material, we present details of the implementation of the dynamics of the IRTP model and estimates of the critical point and the critical exponents of the site percolation transition and the phase separation transitions. We also provide the estimate of the relaxation time and autocorrelation time of the model.

## I. SIMULATION METHOD

The interacting run-and-tumble particle (IRTP) model is similar to the conserved lattice gas (CLG) model on a square lattice with attractive interaction strength  $J$  (and temperature set to  $T = 1$ ). However, in the IRTP model, particles move asymmetrically to their nearest neighbors. Each particle possesses an internal orientation pointing toward one of its nearest neighbors and preferentially moves in that direction more frequently than in the other three. The movement occurs with a directional probability ratio of  $1:p:p:p$ , governed by the Metropolis rate, as in the CLG model.

Additionally, particles can “tumble”—that is, change their internal orientation—with rate  $\omega$ . The parameter  $\omega$  controls the persistence of motion along the internal orientation; hence,  $\omega^{-1}$  can be interpreted as a measure of motility. The directional asymmetry parameter  $p$  introduces translational diffusion into the dynamics of these motile run-and-tumble particles. A schematic illustration of the dynamics is shown in the main text (Fig. 2).

This system violates detailed balance and exhibits a non-equilibrium phase separation transition, which is discussed in detail in the main text. In the following, we present the Monte Carlo (MC) simulation algorithm used for simulating the IRTP model. At each step of the MC sweep, a particle  $k$  is chosen randomly and independently from a collection of total  $N$  particles. If this particle occupies a site  $\mathbf{i}$  and if its intrinsic direction is  $\theta$  then it dominantly moves along the direction  $\boldsymbol{\delta}_0 = (\cos(\theta), \sin(\theta))$ , in comparison to other three directions  $\boldsymbol{\delta}_q = (\cos(\theta + q\frac{\pi}{2}), \sin(\theta + q\frac{\pi}{2}))$  with  $q = 1, 2, 3$ . Then, for a small time step  $\Delta t$ , the following events occur with the respective probabilities:

prob.  $r_0\Delta t$ : if  $n_{\mathbf{i}+\boldsymbol{\delta}_0} = 0$ ;  $n_{\mathbf{i}} = 0, n_{\mathbf{i}+\boldsymbol{\delta}_0} = 1$

prob.  $r_1p\Delta t$ : if  $n_{\mathbf{i}+\boldsymbol{\delta}_1} = 0$ ;  $n_{\mathbf{i}} = 0, n_{\mathbf{i}+\boldsymbol{\delta}_1} = 1$

prob.  $r_2p\Delta t$ : if  $n_{\mathbf{i}+\boldsymbol{\delta}_2} = 0$ ;  $n_{\mathbf{i}} = 0, n_{\mathbf{i}+\boldsymbol{\delta}_2} = 1$

prob.  $r_3p\Delta t$ : if  $n_{\mathbf{i}+\boldsymbol{\delta}_3} = 0$ ;  $n_{\mathbf{i}} = 0, n_{\mathbf{i}+\boldsymbol{\delta}_3} = 1$

prob.  $\omega\Delta t/3$ :  $\theta \rightarrow \theta + \frac{\pi}{2}$

prob.  $\omega\Delta t/3$ :  $\theta \rightarrow \theta + \pi$

prob.  $\omega\Delta t/3$ :  $\theta \rightarrow \theta + \frac{3\pi}{2}$

where

$$r_q = \begin{cases} 0 & \text{if target site } \mathbf{i} + \boldsymbol{\delta}_q \text{ is empty} \\ \min(1, e^{-\Delta E_q}) & \text{else} \end{cases}, \quad q = 0, 1, 2, 3$$

and  $\Delta E_q$  is the change in energy, following Eq. (1) of the main text when a particle moves from the site  $\mathbf{i}$  to  $\mathbf{i} + \boldsymbol{\delta}_q$ . Note that, the configuration remains unchanged in  $\Delta t$  time interval with probability  $(1 - (r_0 + r_1p + r_2p + r_3p + \omega))\Delta t$ . Now to calculate any statistical quantity (Binder Cumulant, Order parameters as in Eq. (5) and (2) of main text) it is important that the sampling should begin only after the system has reached steady-state. To determine the time required for that we find the point at which the pair correlation function  $G(r)$  becomes static, then we can take this as “equilibration time”  $\tau_{\text{eq}}$ . The dependence of  $\tau_{\text{eq}}$  with critical parameters such as interaction strength  $J$  and

<sup>\*</sup> ab23rs019@iiserkol.ac.in

<sup>†</sup> sayantan.pdf@iiserkol.ac.in

<sup>‡</sup> pkmohanty@iiserkol.ac.in

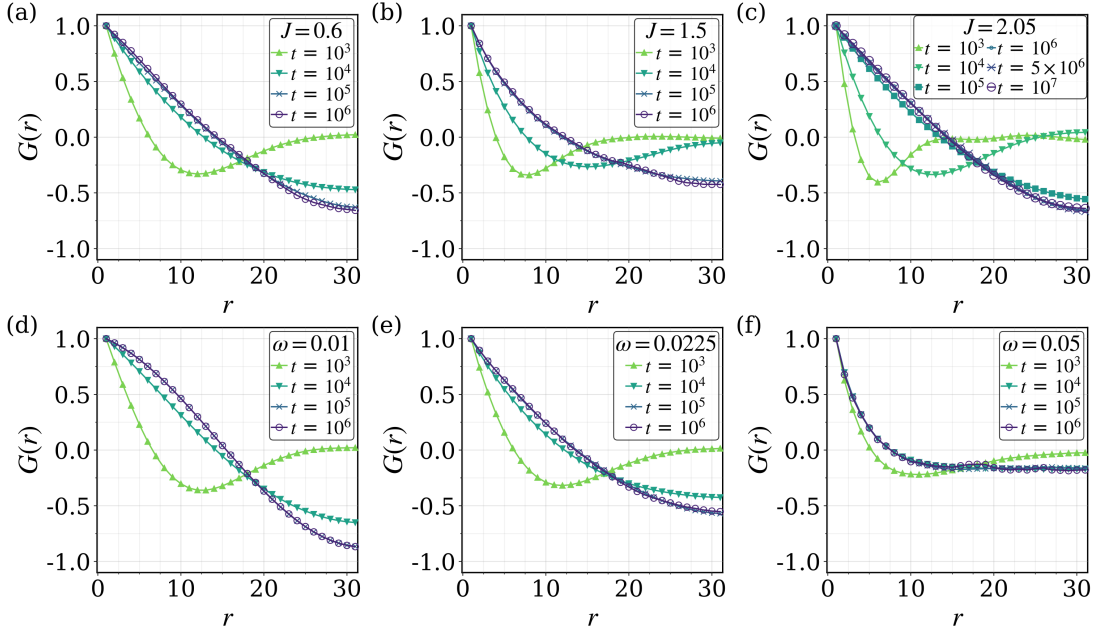

FIG. S1: Determination of equilibration time  $\tau_{\text{eq}}$ : We plotted correlation function  $G(r)$  with  $r$  for system size  $L = 64$ . In plots (a), (b), and (c)  $\omega = 0.02$ , and for three different interaction strengths, we plot  $G(r)$  averaged over at least 100 independent runs as a function of  $r$  for different MC steps. The static nature of  $G(r)$  with respect to time indicates that the system has reached its steady state. For  $J = 0.6$  and  $1.5$ , it is clear that  $t \sim 10^5$  sweeps. Hence, initiating sampling after  $\tau_{\text{eq}} \simeq 10^6$  sweeps should be a good choice, as the system is very likely to have reached a steady state by then. But from Figure (d), for  $J = 2.05$ , the same is nearly  $\tau_{\text{eq}} \simeq 10^7$ . In (d), (e), and (f)  $G(r)$  is plotted for three different tumble rates keeping  $J = 0.6$  fixed. In all cases, it is safe to assume  $\tau_{\text{eq}} \simeq 10^6$ .

tumbling rate  $\omega$  is depicted in supplementary Figure (Fig.) S1. From the figure, one important thing to note is how the equilibration time  $\tau_{\text{eq}}$  increases with increasing interaction strength and thereby it becomes difficult to increase system size for statistical study as one reaches a high  $J$  value.

In the determination of any statistical quantity, another important thing to take care of is that the samples collected are statistically independent. To ensure this, we then calculated the auto-correlation function of the order parameter  $\phi$  (Eq. (5) of main text). From Fig. S2 we can see that the auto-correlation time  $\tau_a$  for system size  $L = 64$  for different interaction strengths.

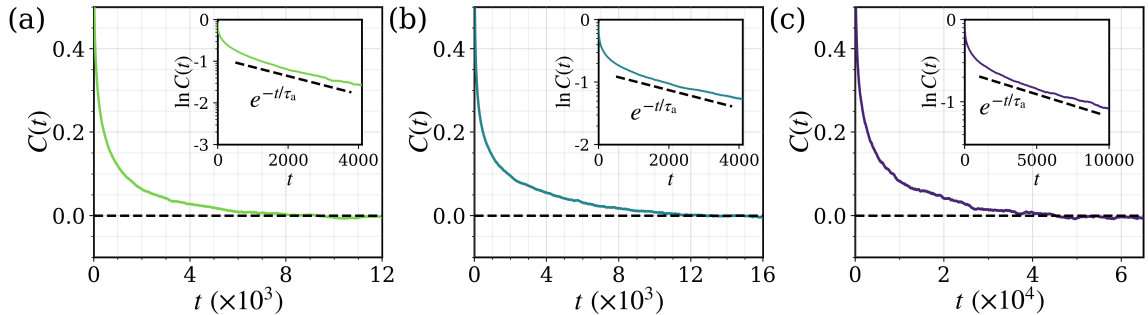

FIG. S2: Determination of auto-correlation time  $\tau_a$ : Figure shows auto-correlation  $C(t)$  of order parameter  $\phi$ . (a) Corresponds to  $J = 0.6$ , from a power law fit of  $e^{-t/\tau_a}$  we have extracted  $\tau_a = 2000$ , in (b) for  $J = 1.5$  we got  $\tau_a = 3000$ , and for (c) corresponding to  $J = 2.05$ , we obtained  $\tau_a = 8000 \sim 10^4$ . So we have taken the time after which two samples can be considered to be statistically independent as  $\tau = 10 \times \tau_a$ .

## II. CRITICAL EXPONENTS OF PERCOLATION STUDY

In the percolation study of the RTP system, we obtained the static exponents  $\nu, \beta$ , and  $\gamma$  (given in Table I of main text) using the finite size scaling analysis (Eq. (8) of main text) of standard percolation order parameter  $\phi = \frac{1}{L^2} \langle s_{\max} \rangle$ . Here the largest cluster size at steady state is determined using an efficient union-find method [1, 2]. In the determination of  $\langle s_{\max} \rangle$  at least 200 independent runs have been taken making sure that in each run the system is well relaxed up to  $\tau_{\text{eq}}$  and then samples are collected at an interval of auto-correlation  $\tau_a$  time. After collecting the samples then various statistics has been calculated with their mean and higher moments and respective uncertainties following standard Jackknife procedure [3]. One thing to note here is that for weak interaction strength system size considered are  $L = 48, 64, 96, 128$ , but as the interaction get stronger we can reach up to 96 due to increasing  $\tau_{\text{eq}}$  and  $\tau_a$ . In main text we have shown FSS collapse figure corresponding to  $J = 0.6$ , here we present other critical points and static exponents corresponding to other interaction strengths.

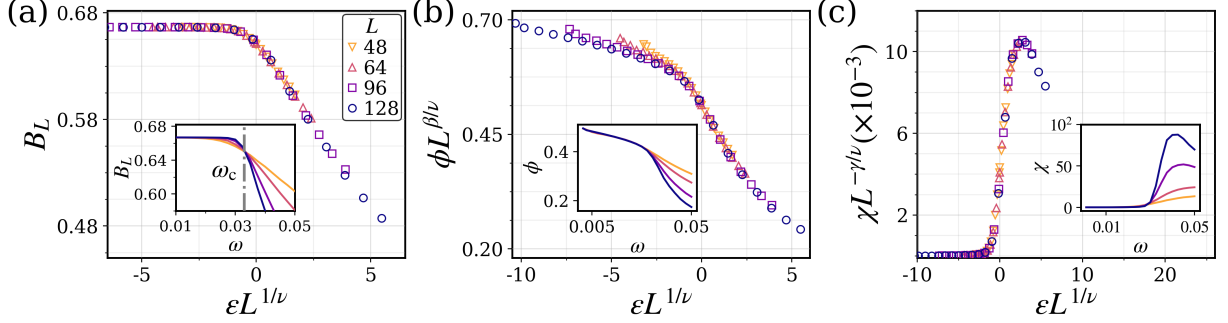

FIG. S3: Critical point ( $\omega_c = 0.0330(2)$ ,  $J_c = 0.00(0)$ ): (a)  $B_L$ , (b)  $\phi$ , (c)  $\chi$ , as function of  $L^{1/\nu}$ . Same quantities are plotted as function of  $\omega$  in insets. Exponents resulted from best scaling collapse are  $\nu = 0.84(1)$ ,  $\beta = 0.058(3)$  and  $\gamma = 1.576(13)$ .

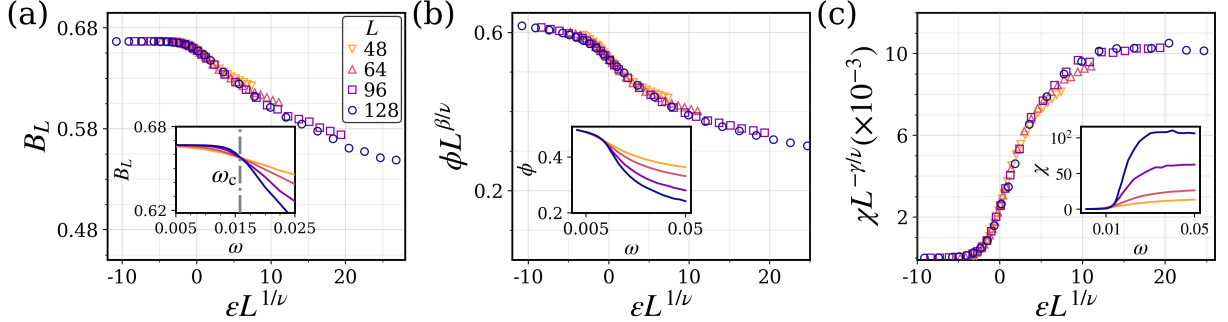

FIG. S4: Critical point ( $\omega_c = 0.0158(2)$ ,  $J_c = 1.20(0)$ ): (a)  $B_L$ , (b)  $\phi$ , (c)  $\chi$ , as function of  $L^{1/\nu}$ . Same quantities are plotted as function of  $\omega$  in insets. Exponents resulted from best scaling collapse are  $\nu = 0.72(2)$ ,  $\beta = 0.033(1)$ , and  $\gamma = 1.374(21)$ .

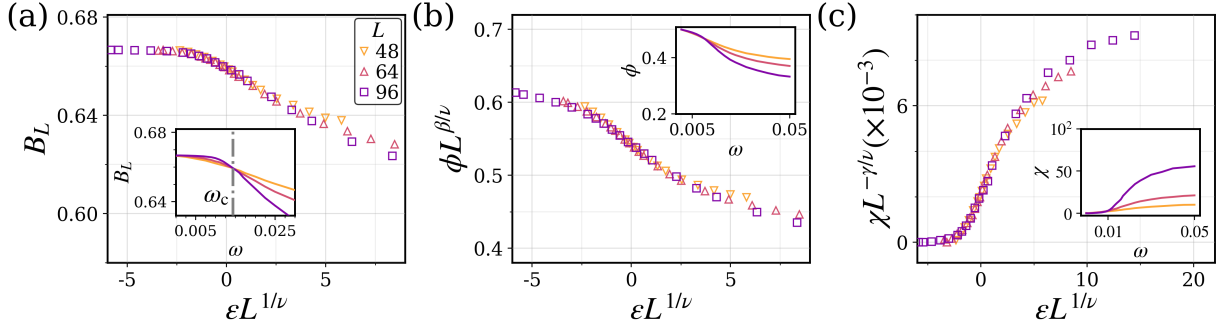

FIG. S5: Critical point ( $\omega_c = 0.0144(4)$ ,  $J_c = 1.50(0)$ ): (a)  $B_L$ , (b)  $\phi$ , (c)  $\chi$ , as function of  $L^{1/\nu}$ . Same quantities are plotted as function of  $\omega$  in insets. Exponents resulted from best scaling collapse are  $\nu = 0.76(3)$ ,  $\beta = 0.034(1)$ , and  $\gamma = 1.452(31)$ .

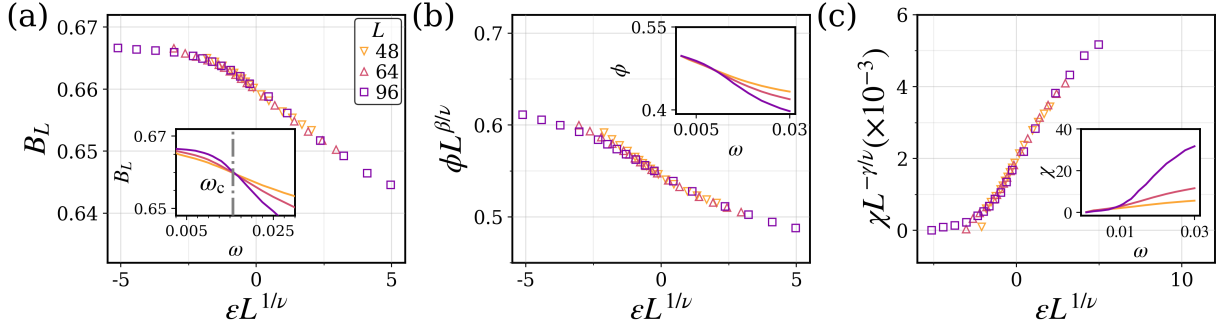

FIG. S6: Critical point ( $\omega_c = 0.0157(2)$ ,  $J_c = 1.70(0)$ ): (a)  $B_L$ , (b)  $\phi$ , (c)  $\chi$ , as function of  $L^{1/\nu}$ . Same quantities are plotted as function of  $\omega$  in insets. Exponents resulted from best scaling collapse are  $\nu = 0.78(3)$ ,  $\beta = 0.035(2)$ , and  $\gamma = 1.490(32)$ .

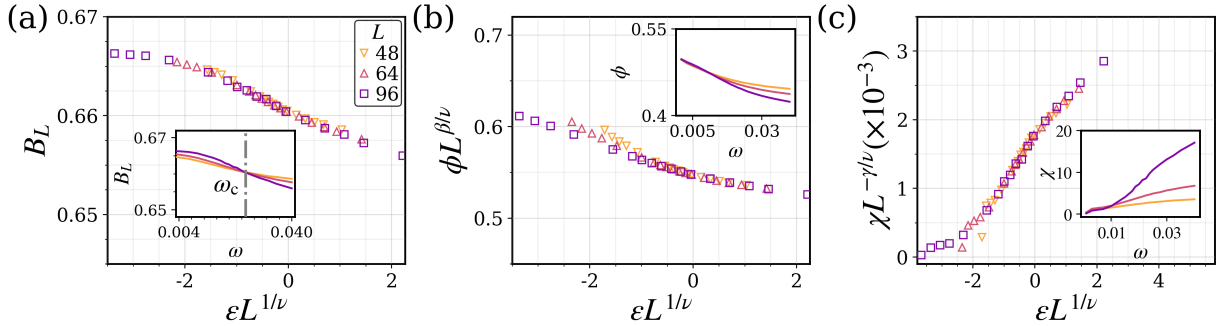

FIG. S7: Critical point ( $\omega_c = 0.0253(2)$ ,  $J_c = 1.90(0)$ ): (a)  $B_L$ , (b)  $\phi$ , (c)  $\chi$ , as function of  $L^{1/\nu}$ . Same quantities are plotted as function of  $\omega$  in insets. Exponents resulted from best scaling collapse are  $\nu = 0.91(2)$ ,  $\beta = 0.043(2)$ , and  $\gamma = 1.734(22)$ .

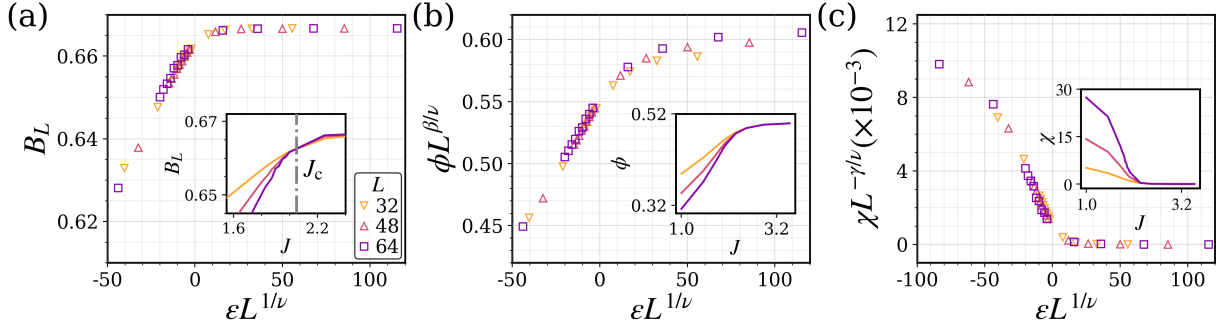

FIG. S8: Critical point ( $\omega_c = 0.0500(0)$ ,  $J_c = 2.05(2)$ ): (a)  $B_L$ , (b)  $\phi$ , (c)  $\chi$ , as function of  $L^{1/\nu}$ . The same quantities are plotted as a function of  $J$  in insets. Exponents resulted from best scaling collapse are  $\nu = 0.95(2)$ ,  $\beta = 0.044(2)$ , and  $\gamma = 1.812(40)$ .

### III. CRITICAL EXPONENTS OF MIPS TRANSITION

For the study of MIPS transition, we have used the order parameter  $\tilde{\phi}$  (Eq. (2) of main text). For further FSS study with this order parameter, we need steady-state samples of  $\tilde{\phi}$ , for that we have taken at least 1000 independent runs, in each run the system is first relaxed up to  $\tau_{eq}$  and then samples are collected with an interval  $\tau_a$ .

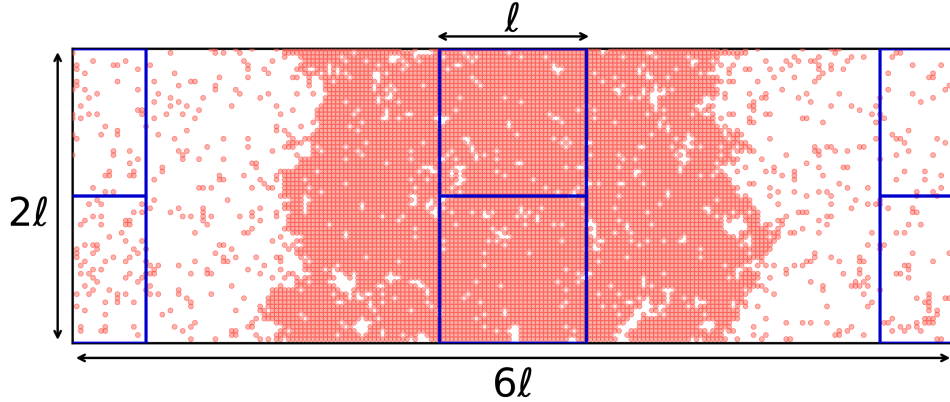

FIG. S9: Snapshot of IRTP system for  $\omega = 0.015$  and  $J = 0.0$ , created in a  $6\ell \times 2\ell$  simulation box where  $\ell = 36$ . The four square sub-boxes each of side length  $\ell$  are placed for efficient sampling of the density (particle number) of liquid and gas phases.

We then followed Jackknife for the determination of any statistical quantity with their respective uncertainties. In the main text we have shown the critical point and corresponding exponents of MIPS transition at  $J_c = 0.6$ . Here we have shown some more critical points and their corresponding exponents, and we also checked for them if the relation given in Eq. (10) in main text holds correctly.

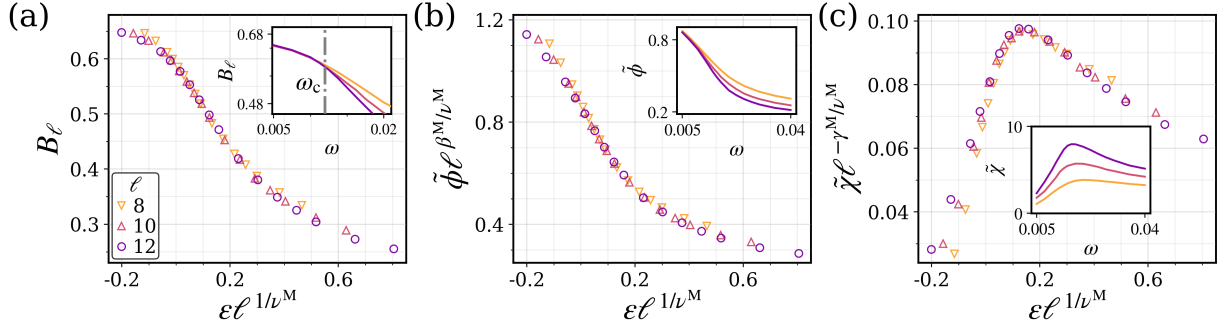

FIG. S10: Critical point ( $\omega_c = 0.012(2)$ ,  $J_c = 1.50(0)$ ), estimated from MIPS order parameter  $\tilde{\phi}$ . (a)  $B_\ell$ , (b)  $\tilde{\phi}$ , (c)  $\chi$ , as function of  $\ell^{1/\nu^M}$  are plotted respectively, where  $\varepsilon = \omega - \omega_c$ . The same quantities are plotted as a function of  $\omega$  in insets. Exponents resulted from best scaling collapse are  $\nu^M = 0.74(4)$ ,  $\beta^M = 0.085(6)$ , and  $\gamma^M = 1.31(8)$ . Following Eq. (9) of main text we can see that the corresponding exponents from the percolation study, are matching well with these results within the margin of error.

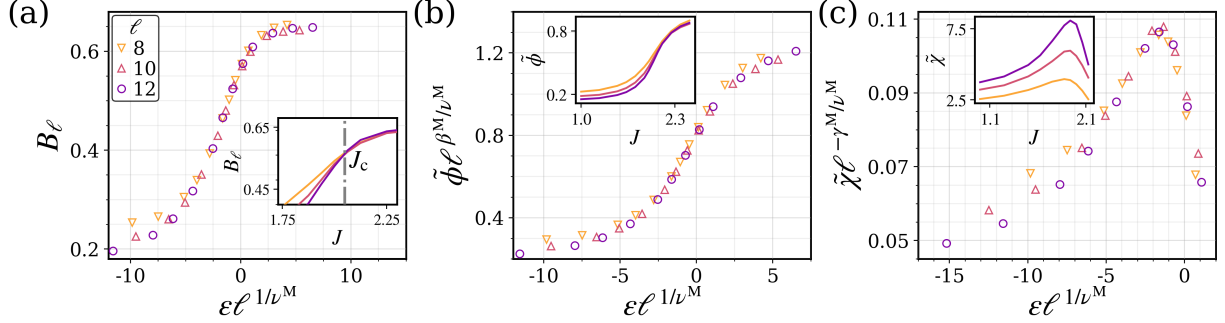

FIG. S11: Critical point ( $\omega_c = 0.050(0)$ ,  $J_c = 2.05(2)$ ), estimated from MIPS order parameter  $\tilde{\phi}$ . In (a)  $B_\ell$ , (b)  $\tilde{\phi}$ , (c)  $\tilde{\chi}$ , as function of  $\ell^{1/\nu^M}$  are plotted respectively where  $\varepsilon = J - J_c$ . The same quantities are plotted as a function of  $J$  in respective insets. Exponents resulted from best scaling collapse are  $\nu^M = 0.93(3)$ ,  $\beta^M = 0.120(2)$ , and  $\gamma^M = 1.62(6)$ . Following Eq. (9) of main text we can see that the corresponding exponents from the percolation study, are matching well with these results within the margin of error.

- 
- [1] M. E. J. Newman and R. M. Ziff, Efficient monte carlo algorithm and high-precision results for percolation, *Phys. Rev. Lett.* **85**, 4104 (2000).
  - [2] M. E. J. Newman and R. M. Ziff, Fast monte carlo algorithm for site or bond percolation, *Physical Review E* **64**, 10.1103/physreve.64.016706 (2001).
  - [3] B. Efron, *The Jackknife, the Bootstrap and Other Resampling Plans* (Society for Industrial and Applied Mathematics, 1982).
